# Supplementary material for: Sonic: Fast and Transferable Data Poisoning on Clustering Algorithms
Source: arXiv:2408.07558 source file (2024-08-14)
Supplement: Supplementary file 1 [file additional_experiments.tex]

\section{Additional Experiments}
In Figure~\ref{fig:full_robustness_analysis}, we include the regression lines for all the \sonic configurations with different FISHDBC approximation levels \ef. Lower \ef values in FISHDBC can widen the gap between \slowPoison and \sonic, slightly reducing benchmarking accuracy in exchange for lower execution times.
\begin{figure}[ht]
    \centering
    \includegraphics[width=0.49\textwidth]{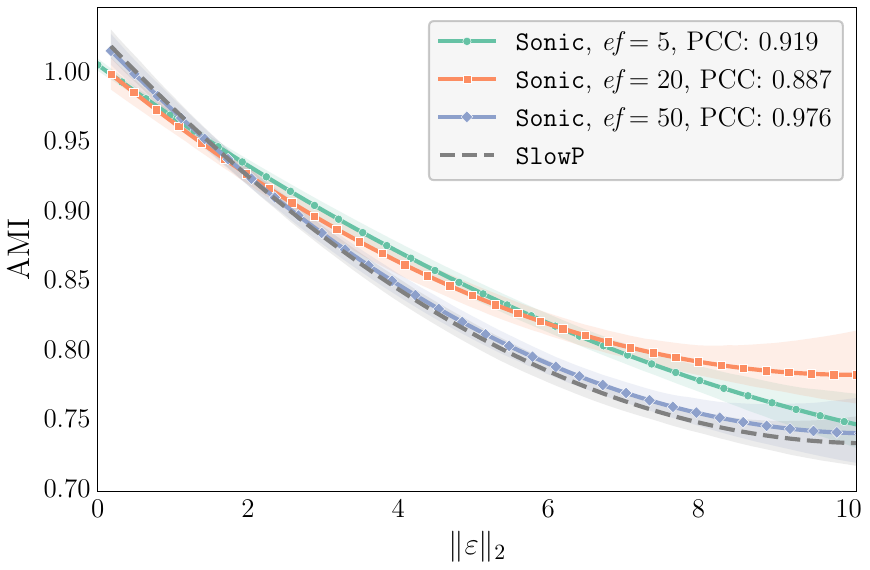}
    \includegraphics[width=0.49\textwidth]{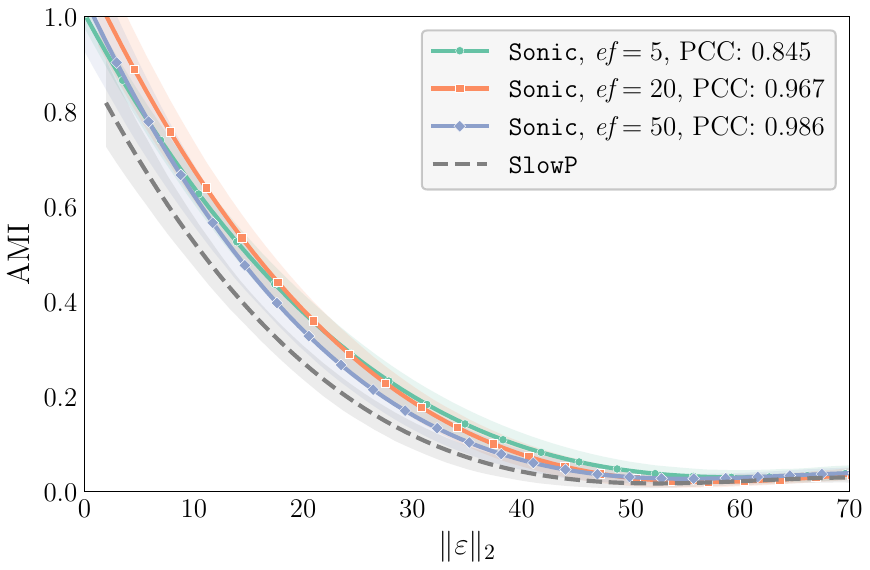}
    \includegraphics[width=0.49\textwidth]{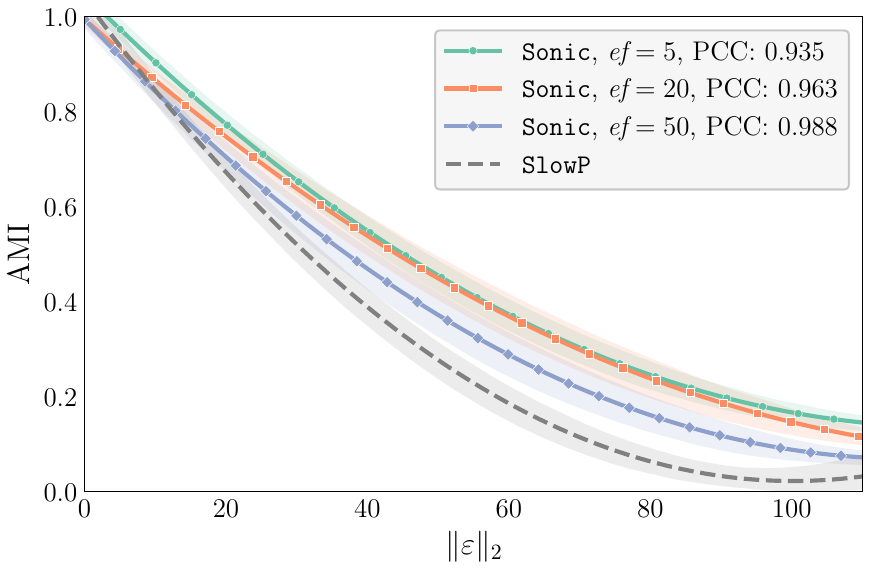}
    \includegraphics[width=0.49\textwidth]{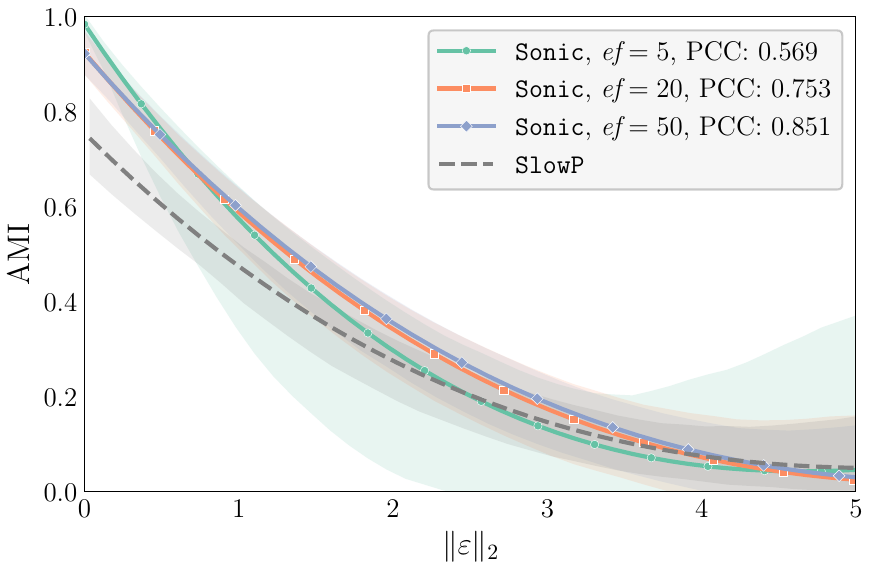}
    \caption{Regression lines of the Robustness analysis on 20 Newsgroups (top-left), MNIST (top-right), FASHIONMNIST (bottom-left) and CIFAR-10 (bottom-right). We display \sonic at various FISHDBC approximation levels. For 20 Newsgroups, we display both overall AMI and AMI specific to the victim-target cluster.}
    \label{fig:full_robustness_analysis}
\end{figure}
